# Supplementary material for: Second-Order Optimization for Non-Convex Machine Learning: An Empirical Study
Source: arXiv:1708.07827 source file (2018-02-16)
Supplement: Supplementary file 1 [file appendix.tex]

%\section{Synthetic Dataset} 
%\label{sec:example_synthetic}
%In this section, we further highlight the advantages of non-uniform sampling over simple uniform sampling  for TR (Algorithm \ref{alg:STR_fg}) and ARC (Algorithm \ref{alg:SCR_fg}) discussed in Section~\ref{sec:subsampled_TR_CR}. 
%
%\paragraph{Data Generation} We set $n = 100,000, d=100$, choose a ``true'' parameter $\x^{*} \in \bbR^d$ as a vector of all $ 1 $'s, and then generate features, $\a_i$, from multivariate Student's t-distribution with correlation matrix $ \Sigma $ and 1 degree of freedom. We also generate the corresponding labels $y_i\in\{0,1\}$ as $y_i = \mathbf{1}_{\{ \phi(\lin{\a_i, \x^{*}}) > 0.5 \}}$. To further introduce non-uniformity, i.e., incoherence, in the data set, we choose the correlation matrix, $ \Sigma \in \mathbb{R}^{d \times d}$ as $\Sigma_{ij} = 2^{1-|i-j|}$.
%In the same way, we also generate $ 100,000 $ data points with their corresponding labels as test set, on which we evaluate the generalization performance. 
%
%For both TR (Algorithm \ref{alg:STR_fg}) and ARC (Algorithm \ref{alg:SCR_fg}), we compare uniform and non-uniform sampling, as well as the corresponding deterministic algorithms in which the exact Hessian is used at every iteration. For this, we plot the training loss as well as the test classification accuracy vs number of propagations (calculated as described earlier). All algorithms, starting from the same initial point generated from multivariate standard normal, are run for 200 iterations. Results are depicted in Figure~\ref{fig:uni_nonuni_comparison}. 
%
%\begin{figure}[H]
%\centering
%\mbox{
%\addtocounter{subfigure}{-1}
%\subfigure{
%	\includegraphics[scale = 0.39]{figs/blc_test_data/test_T1/legend_TR.png}
%}
%\subfigure[]{
%\includegraphics[scale = 0.39]{figs/blc_test_data/test_T1/tr_T1_noProps_tr_tr_loss.png}\label{fig:1a_tr}
%}
%\subfigure[]{
%\includegraphics[scale = 0.39]{figs/blc_test_data/test_T1/tr_T1_noProps_tr_te_acc.png}\label{fig:1b_tr}
%}}
%\mbox{
%\hspace{-2mm} \addtocounter{subfigure}{-1}
%\subfigure{
%	\includegraphics[scale = 0.39]{figs/blc_test_data/test_T1/legend_ARC.png}
%}
%\subfigure[]{
%	\includegraphics[scale = 0.39]{figs/blc_test_data/test_T1/arc_T1_noProps_tr_tr_loss.png}\label{fig:1a_arc}
%}
%\subfigure[]{
%	\includegraphics[scale = 0.39]{figs/blc_test_data/test_T1/arc_T1_noProps_tr_te_acc.png}\label{fig:1b_arc}
%}}
%\caption{Performances of deterministic and sub-sampled TR and ARC methods based on uniform and non-uniform sampling on the synthetic dataset for the example of Section~\ref{sec:example_synthetic}. ``Full'', ``Uniform'', and ``Non Uniform'', respectively, refer to deterministic algorithm using the entire dataset, uniform and non-uniform sampling. ``$ \# $ of Props'' refer to the total number of propagations computed as described in Section~\ref{sec:experiments}. (a) \& (c) Training loss vs.\ number of propagations, 
%%where both ``$ x  $'' and ``$ y $'' axes are on the logarithmic scale and
% (b) \& (d) test  classification accuracy vs.\ number of propagations 
%% with ``$ x $'' axis drawn on the logarithmic scale. 
%``Percentage'' sign indicates the sub-sampling ratio, i.e., $ |\mathcal{S}|/n $. Note that here x-axes are in logarithmic scale.
%%Note that in all these examples, non-uniform sampling (``green curve'') outperforms all other algorithms, as measured by training error and test accuracy vs total number of propagations.
%\label{fig:uni_nonuni_comparison}}
%\end{figure}
%For such a problem with incoherent data , as it can be seen from Figure~\ref{fig:uni_nonuni_comparison}, non-uniform sampling with only $ 1\% $ sample size can significantly outperform the deterministic algorithm as well as oblivious uniform sampling, as measured by training error and test accuracy vs total number of propagations. This is indeed predicted by~\citet[Lemma 5]{xuNonconvexTheoretical2017} which, for non-uniformly distributed data, can yield a significantly smaller sample size compared to~\citet[Lemma 4]{xuNonconvexTheoretical2017} with uniform sampling. In fact, for this example, uniform sampling with a sample-size of $0.01 n$ or $0.05 n$, is not capable of capturing enough curvature, and indeed, performs worse than fully deterministic counterpart, i.e., with such a sample size, uniformly sub-sampling the Hessian does not offer any computational advantage in this case.
